# Supplementary material for: Electron-phonon coupling and hot electron thermalization in titanium nitride
Source: arXiv:1908.06620 ancillary file (2019-11-08)
Supplement: Supplementary file 1 [file supp-info-TiN.pdf]

# Supporting information for: Electron-phonon coupling and hot electron thermalization in titanium nitride

Stefano Dal Forno<sup>\*,†</sup> and Johannes Lischner<sup>\*,‡</sup>

<sup>†</sup>*Department of Physics, Imperial College London, London SW7 2AZ, United Kingdom.*

<sup>‡</sup>*Department of Physics and Department of Materials, and the Thomas Young Centre for Theory and Simulation of Materials, Imperial College London, London SW7 2AZ, United Kingdom*

E-mail: [tenobaldi@gmail.com](mailto:tenobaldi@gmail.com); [j.lischner@imperial.ac.uk](mailto:j.lischner@imperial.ac.uk)

DFT results for gold and all the TiN systems considered: Au, TiN<sub>0.80</sub>O<sub>0.20</sub>, TiN<sub>0.85</sub>O<sub>0.15</sub>, TiN<sub>0.90</sub>O<sub>0.10</sub>, TiN<sub>0.95</sub>O<sub>0.05</sub>, TiN<sub>1.00</sub>, TiN<sub>0.97</sub>, TiN<sub>0.94</sub>, TiN<sub>0.91</sub>, TiN<sub>0.88</sub>, TiN<sub>0.84</sub>. TiN systems have been ordered with respect to the number of electrons per unit cell.

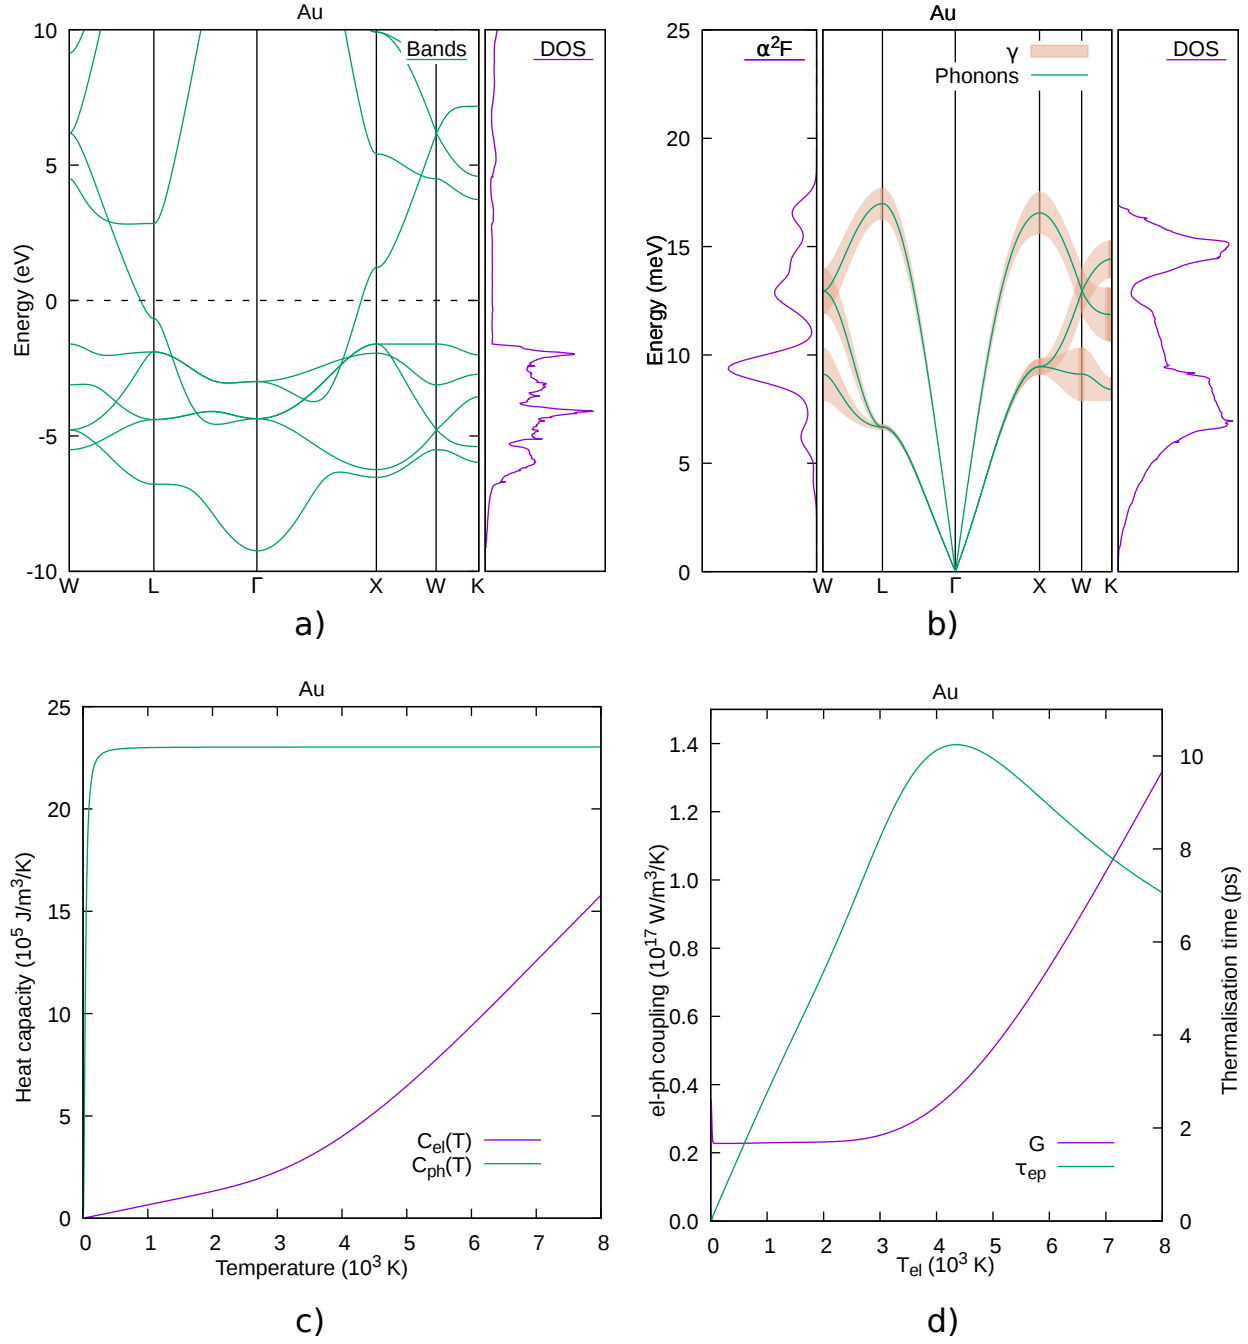

Figure S1: DFT results for Au. a) Electron band structure and DOS (DOS values in the range 0 to 5 states/eV/unitcell). b) Phonon band structure, DOS, phonon linewidths (magnification  $\times 200$ ) and Eliashberg function (DOS and  $\alpha^2F$  in the range 0 to 0.06 states/eV/unitcell and 0 to 0.3, respectively). c) Electron and phonon heat capacities. d) Electron-phonon coupling parameter and hot electron thermalisation time.

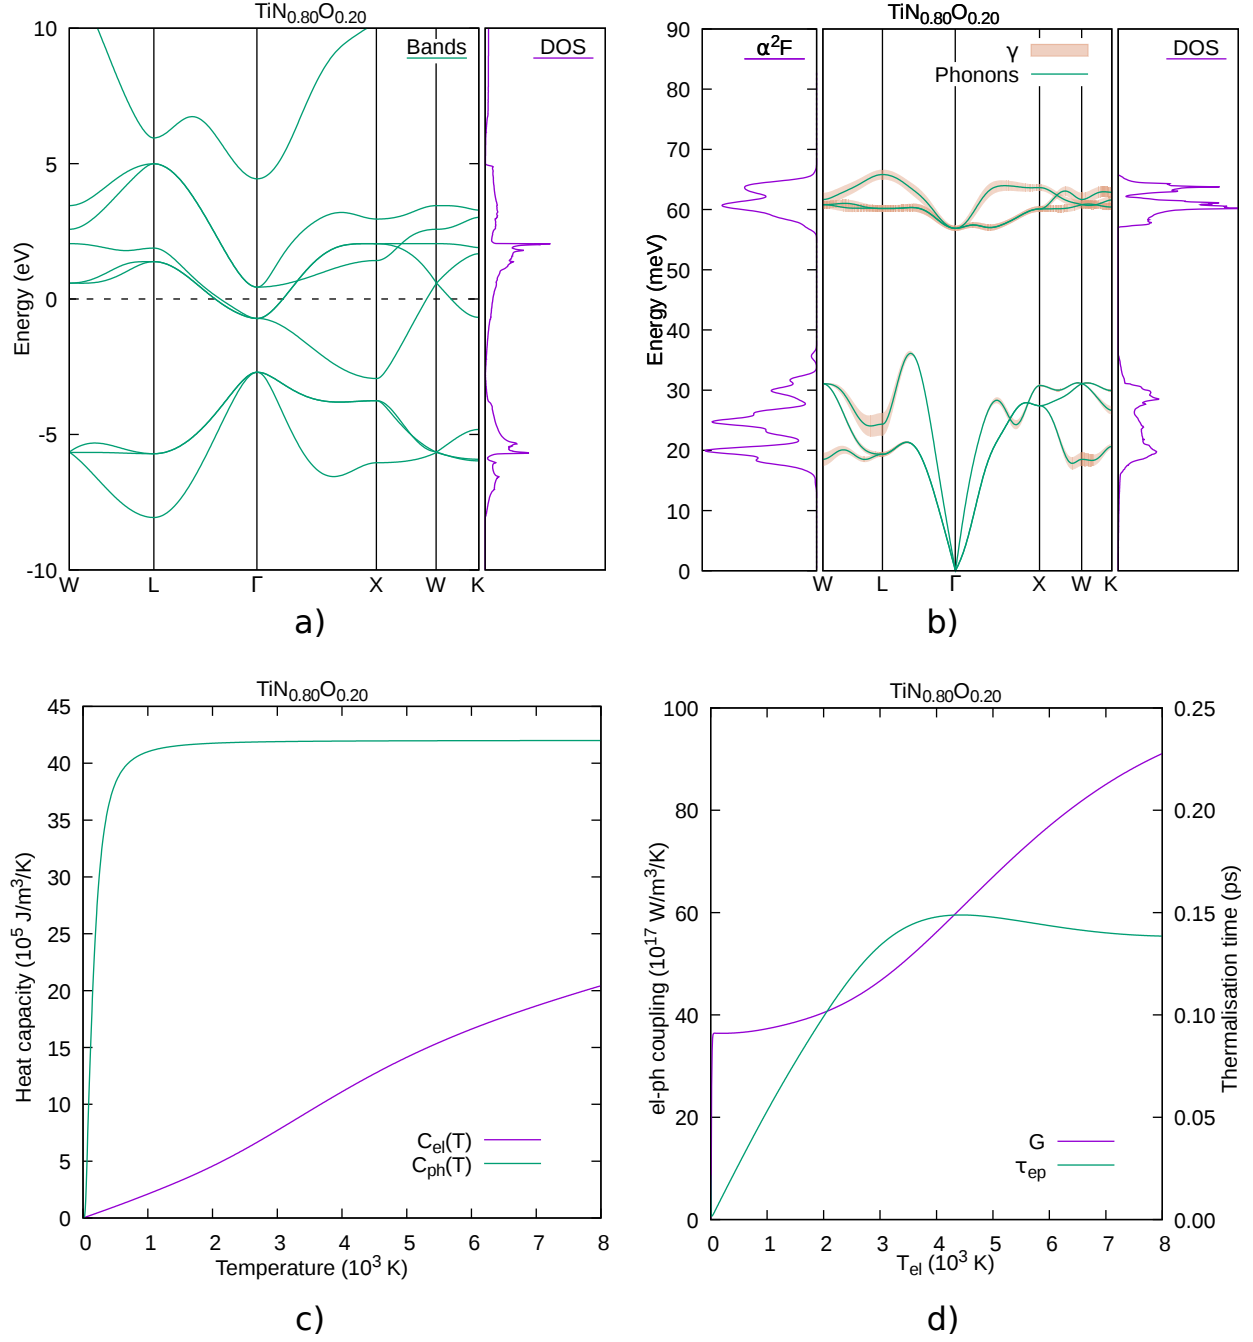

Figure S2: DFT results for  $\text{TiN}_{0.80}\text{O}_{0.20}$ . a) Electron band structure and DOS (DOS values in the range 0 to 16 states/eV/unitcell). b) Phonon band structure, DOS, phonon linewidths (magnification  $\times 2$ ) and Eliashberg function (DOS and  $\alpha^2F$  in the range 0 to 0.12 states/eV/unitcell and 0 to 1.3, respectively). c) Electron and phonon heat capacities. d) Electron-phonon coupling parameter and hot electron thermalisation time.

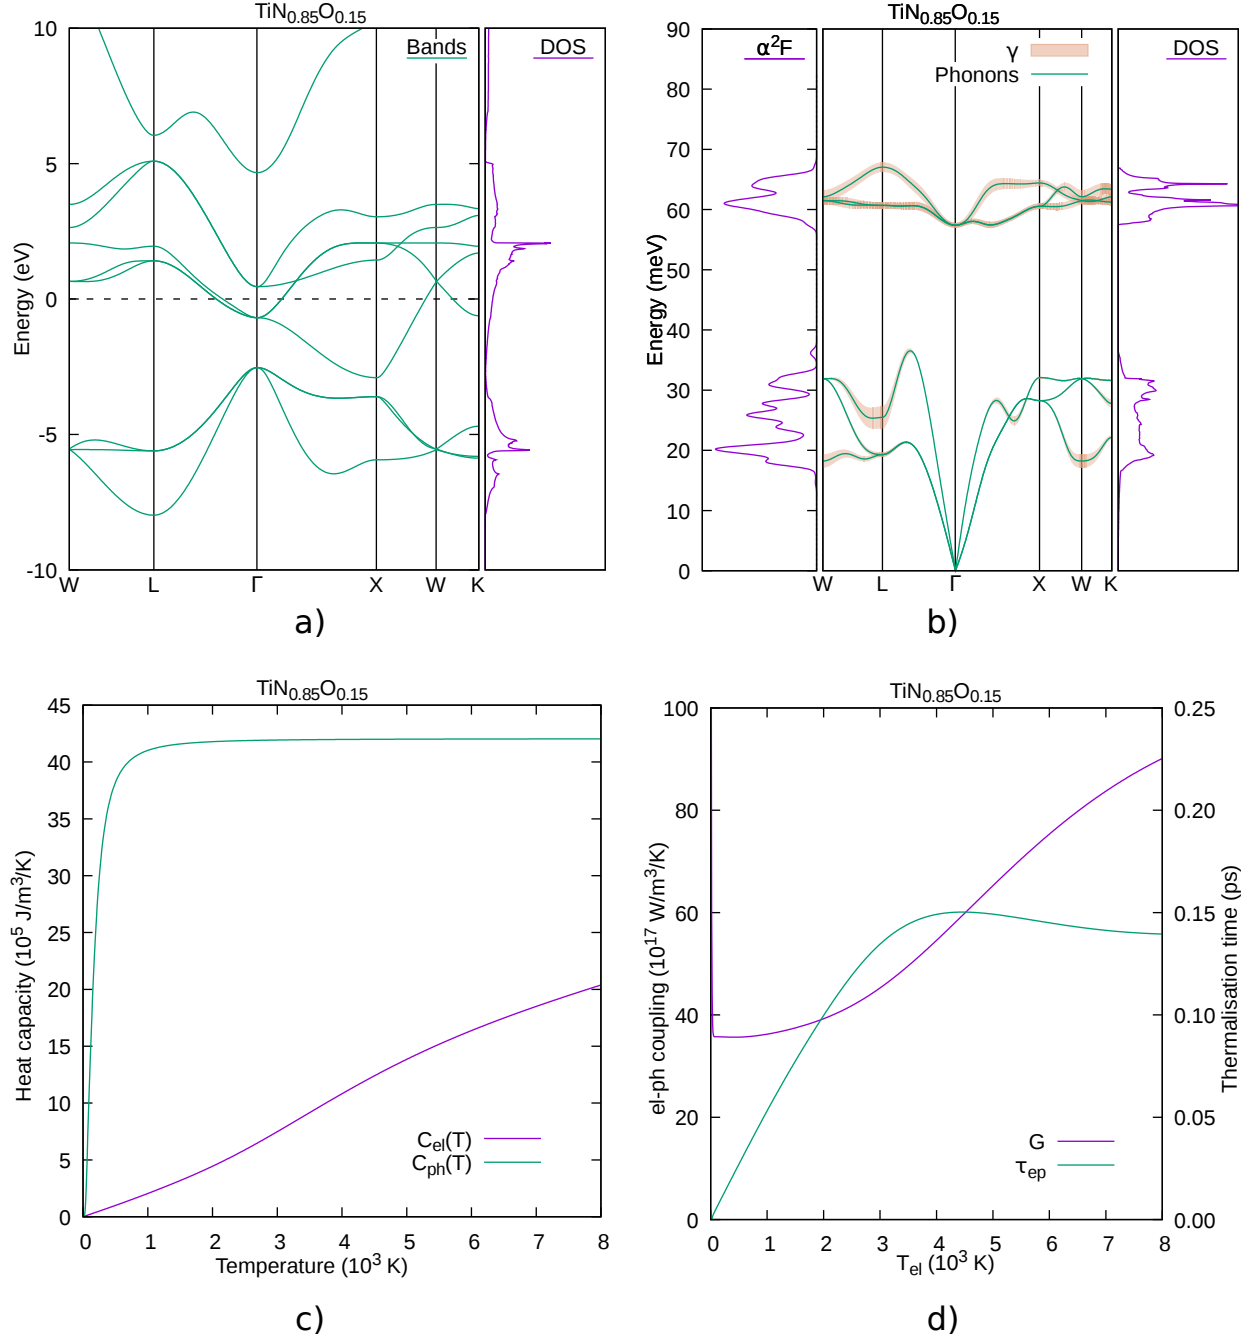

Figure S3: DFT results for  $\text{TiN}_{0.85}\text{O}_{0.15}$ . a) Electron band structure and DOS (DOS values in the range 0 to 16 states/eV/unitcell). b) Phonon band structure, DOS, phonon linewidths (magnification  $\times 2$ ) and Eliashberg function (DOS and  $\alpha^2F$  in the range 0 to 0.12 states/eV/unitcell and 0 to 1.3, respectively). c) Electron and phonon heat capacities. d) Electron-phonon coupling parameter and hot electron thermalisation time.

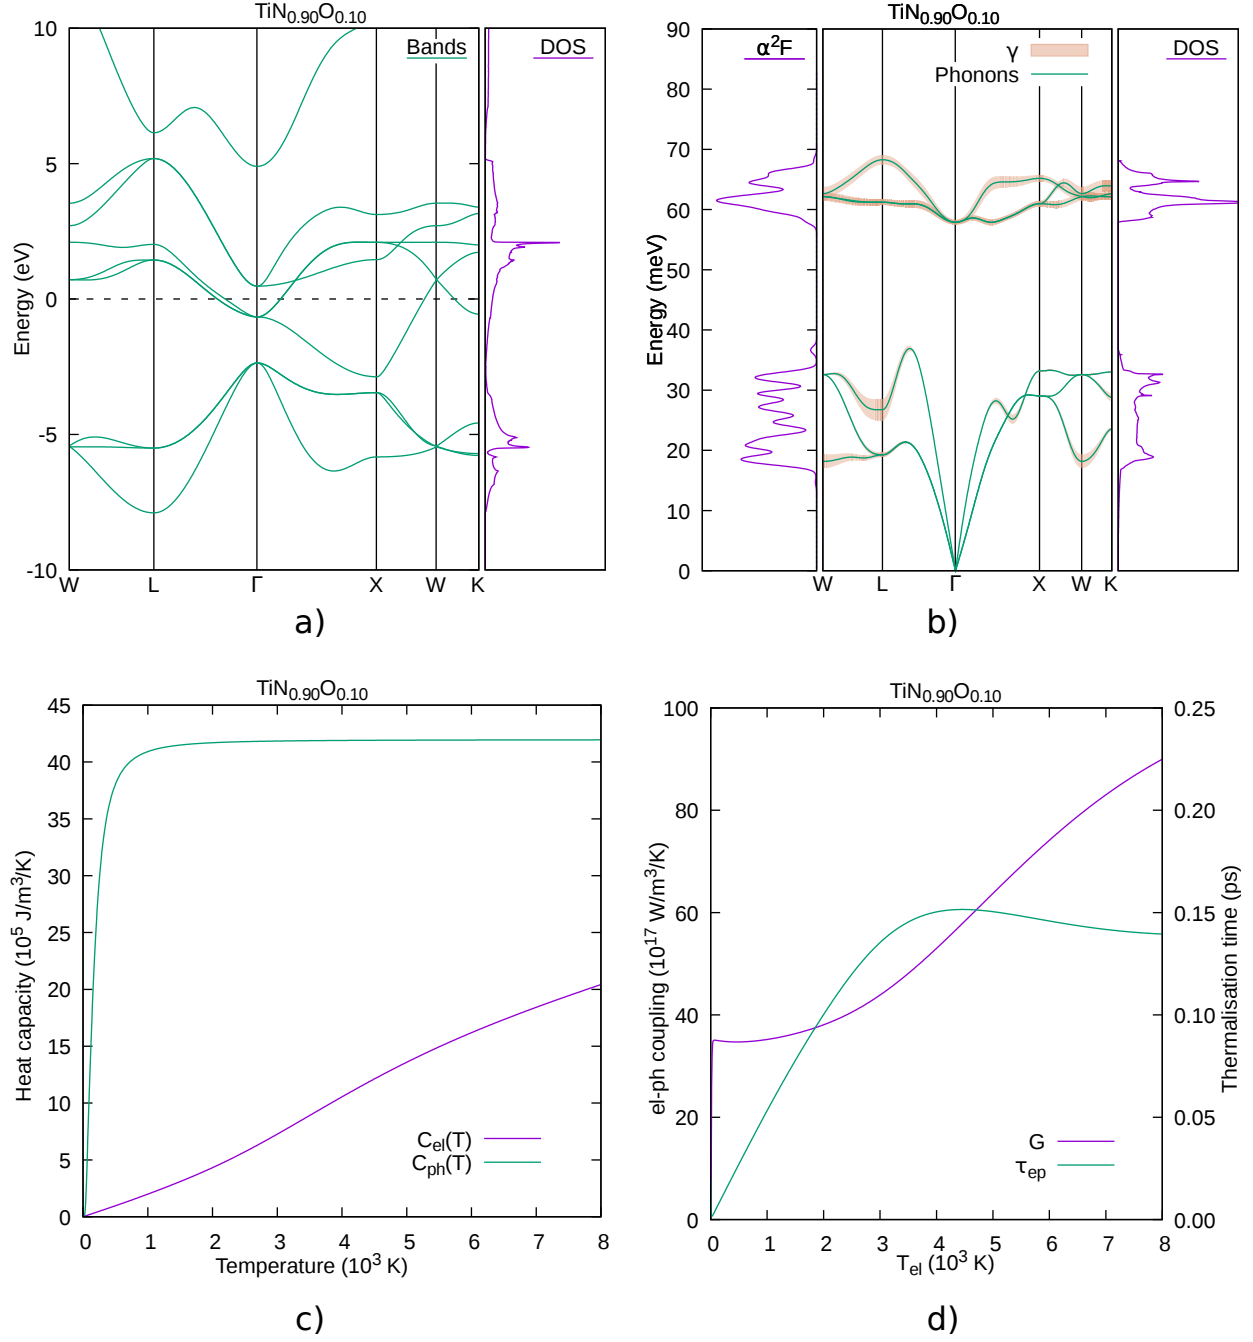

Figure S4: DFT results for  $\text{TiN}_{0.90}\text{O}_{0.10}$ . a) Electron band structure and DOS (DOS values in the range 0 to 16 states/eV/unitcell). b) Phonon band structure, DOS, phonon linewidths (magnification  $\times 2$ ) and Eliashberg function (DOS and  $\alpha^2F$  in the range 0 to 0.12 states/eV/unitcell and 0 to 1.3, respectively). c) Electron and phonon heat capacities. d) Electron-phonon coupling parameter and hot electron thermalisation time.

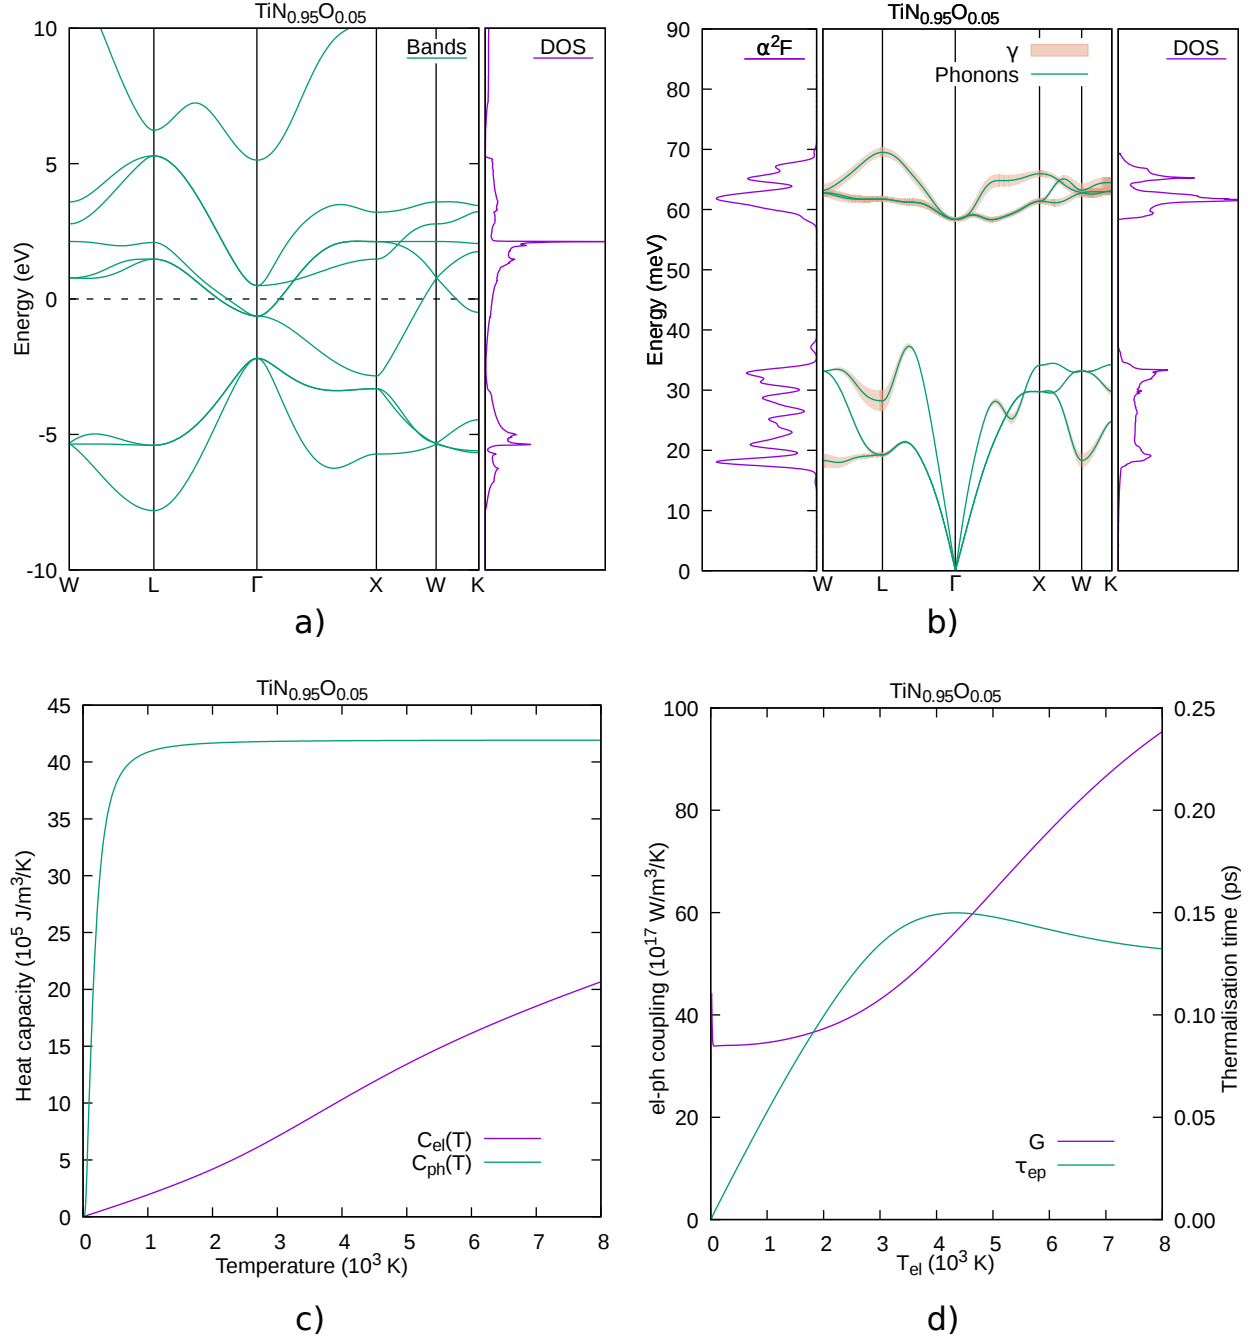

Figure S5: DFT results for  $\text{TiN}_{0.95}\text{O}_{0.05}$ . a) Electron band structure and DOS (DOS values in the range 0 to 16 states/eV/unitcell). b) Phonon band structure, DOS, phonon linewidths (magnification  $\times 2$ ) and Eliashberg function (DOS and  $\alpha^2F$  in the range 0 to 0.12 states/eV/unitcell and 0 to 1.3, respectively). c) Electron and phonon heat capacities. d) Electron-phonon coupling parameter and hot electron thermalisation time.

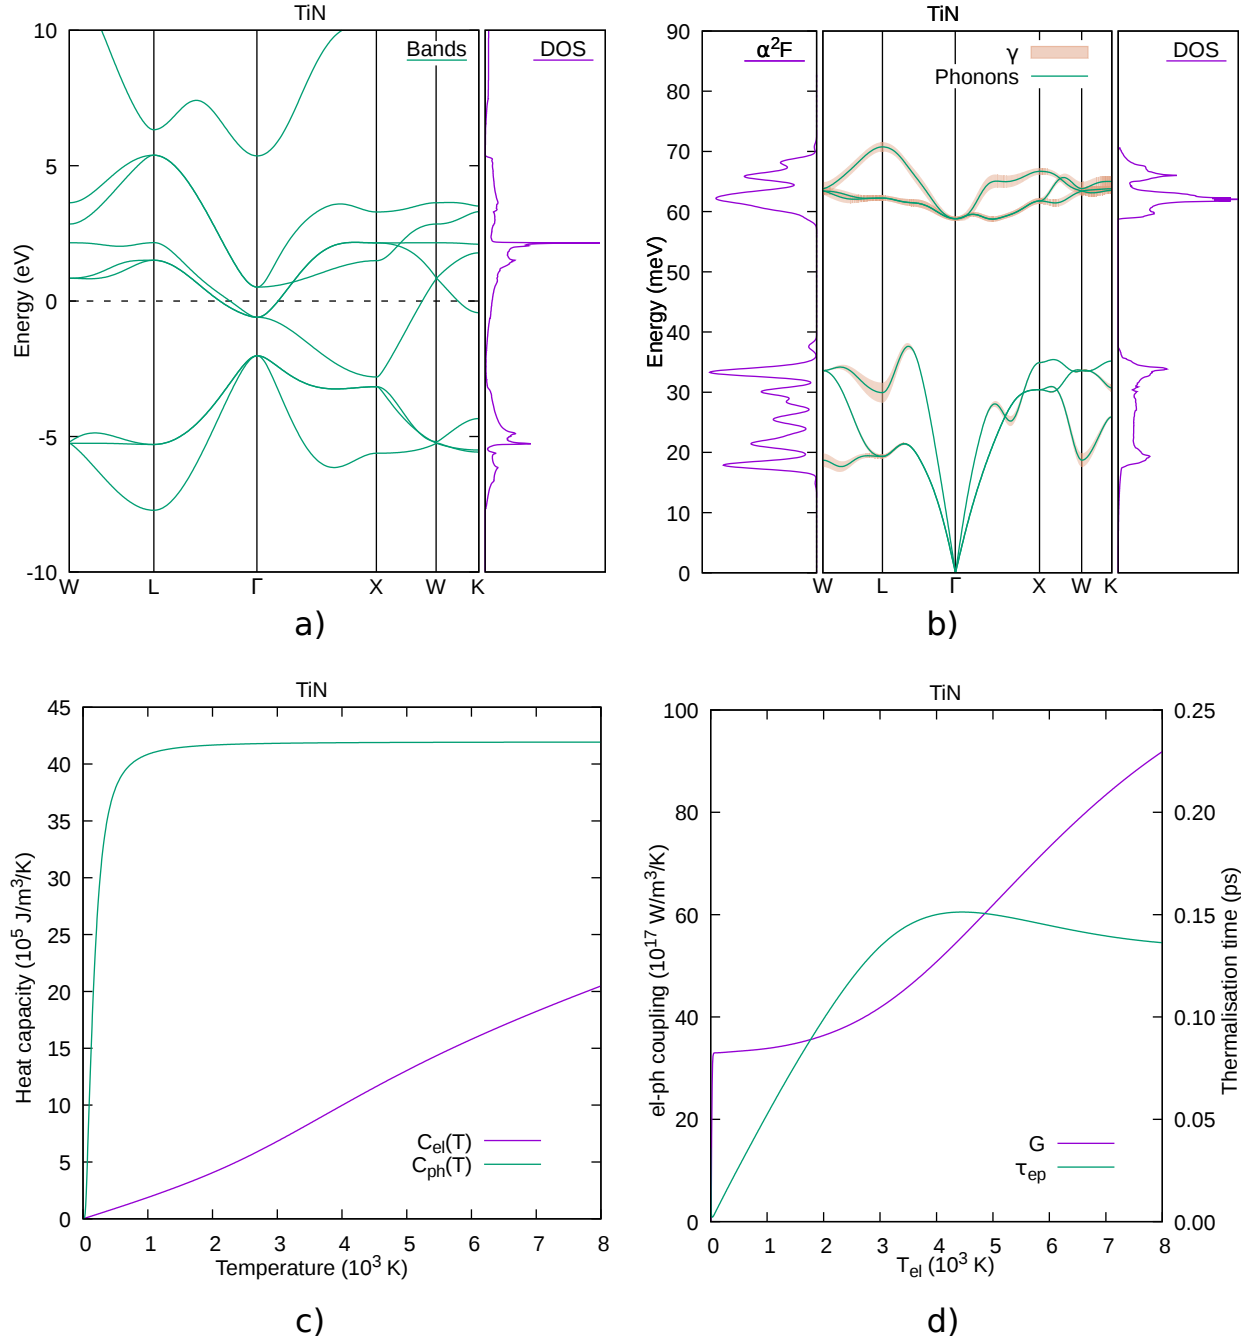

Figure S6: DFT results for TiN. a) Electron band structure and DOS (DOS values in the range 0 to 16 states/eV/unitcell). b) Phonon band structure, DOS, phonon linewidths (magnification  $\times 2$ ) and Eliashberg function (DOS and  $\alpha^2F$  in the range 0 to 0.12 states/eV/unitcell and 0 to 1.3, respectively). c) Electron and phonon heat capacities. d) Electron-phonon coupling parameter and hot electron thermalisation time.

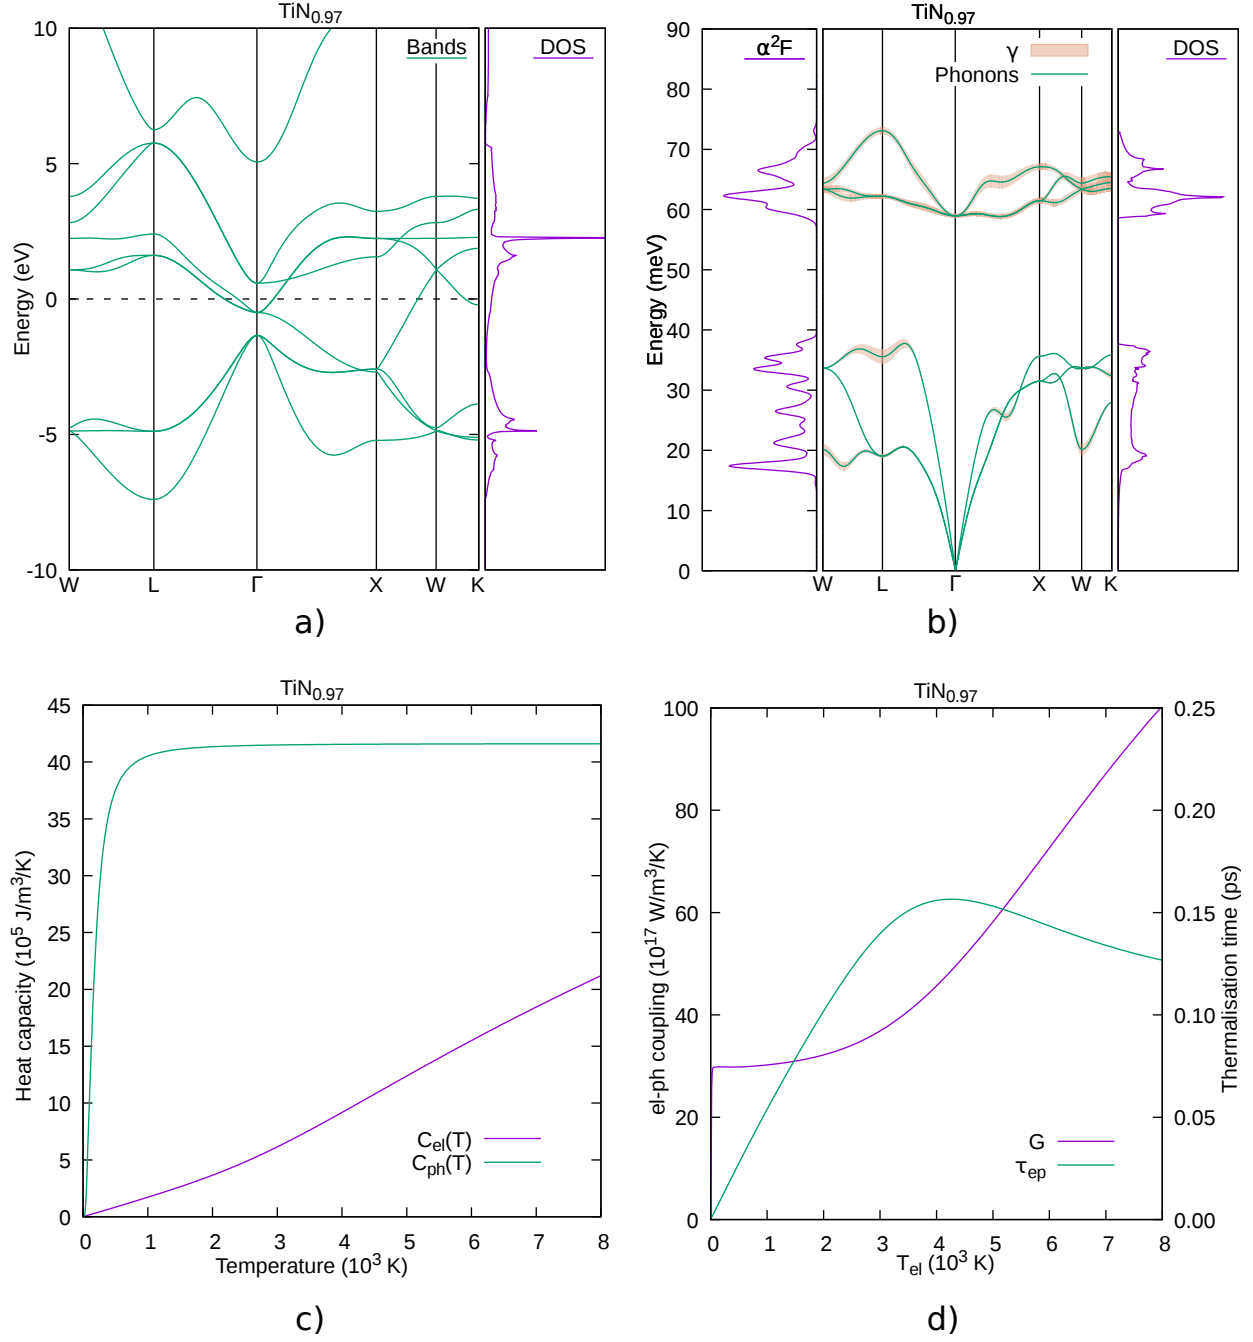

Figure S7: DFT results for  $\text{TiN}_{0.97}$ . a) Electron band structure and DOS (DOS values in the range 0 to 16 states/eV/unitcell). b) Phonon band structure, DOS, phonon linewidths (magnification  $\times 2$ ) and Eliashberg function (DOS and  $\alpha^2F$  in the range 0 to 0.12 states/eV/unitcell and 0 to 1.3, respectively). c) Electron and phonon heat capacities. d) Electron-phonon coupling parameter and hot electron thermalisation time.

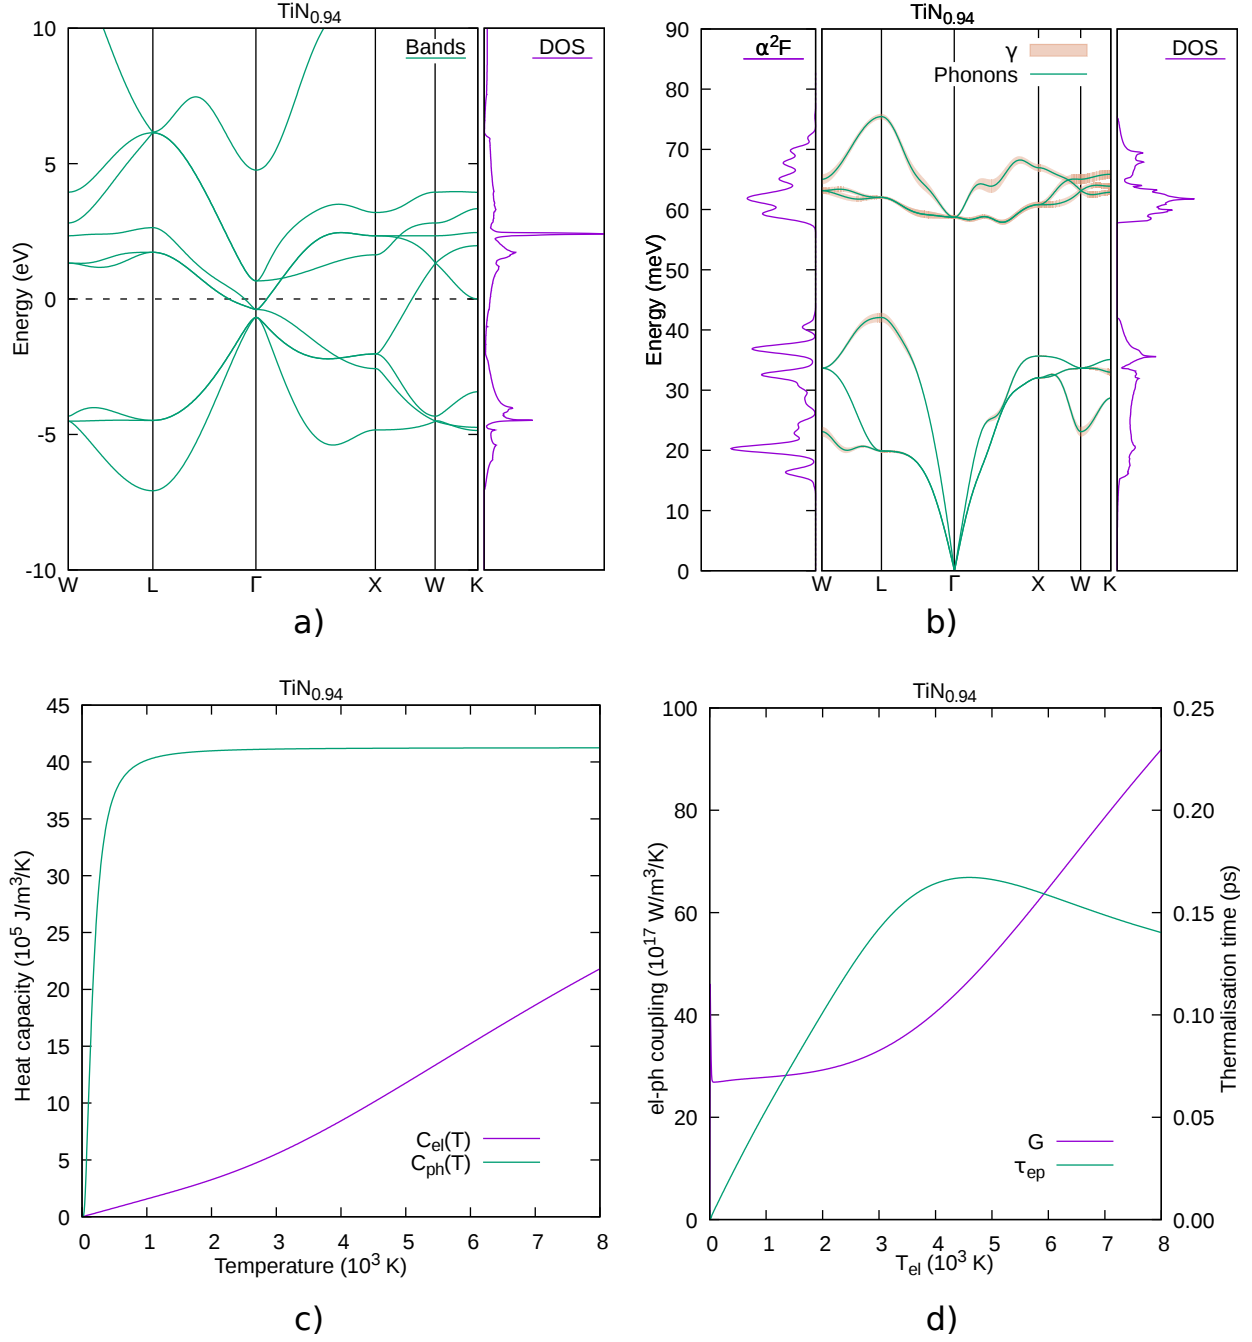

Figure S8: DFT results for  $\text{TiN}_{0.94}$ . a) Electron band structure and DOS (DOS values in the range 0 to 16 states/eV/unitcell). b) Phonon band structure, DOS, phonon linewidths (magnification  $\times 2$ ) and Eliashberg function (DOS and  $\alpha^2F$  in the range 0 to 0.12 states/eV/unitcell and 0 to 1.3, respectively). c) Electron and phonon heat capacities. d) Electron-phonon coupling parameter and hot electron thermalisation time.

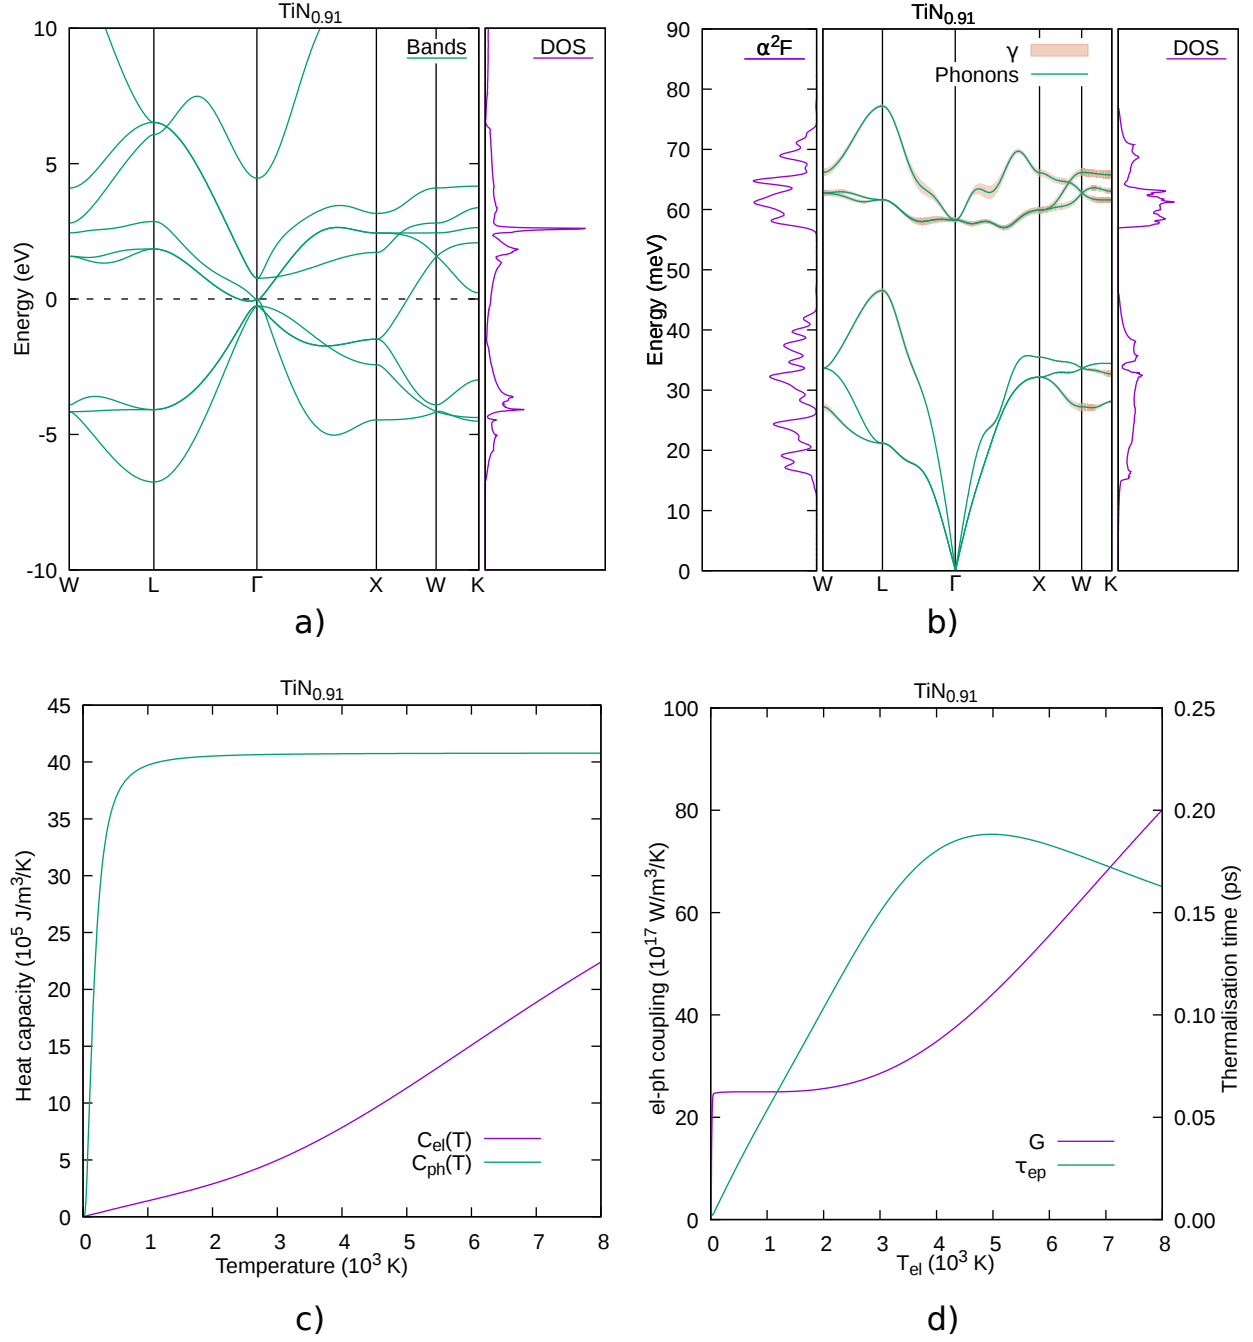

Figure S9: DFT results for  $\text{TiN}_{0.91}$ . a) Electron band structure and DOS (DOS values in the range 0 to 16 states/eV/unitcell). b) Phonon band structure, DOS, phonon linewidths (magnification  $\times 2$ ) and Eliashberg function (DOS and  $\alpha^2F$  in the range 0 to 0.12 states/eV/unitcell and 0 to 1.3, respectively). c) Electron and phonon heat capacities. d) Electron-phonon coupling parameter and hot electron thermalisation time.

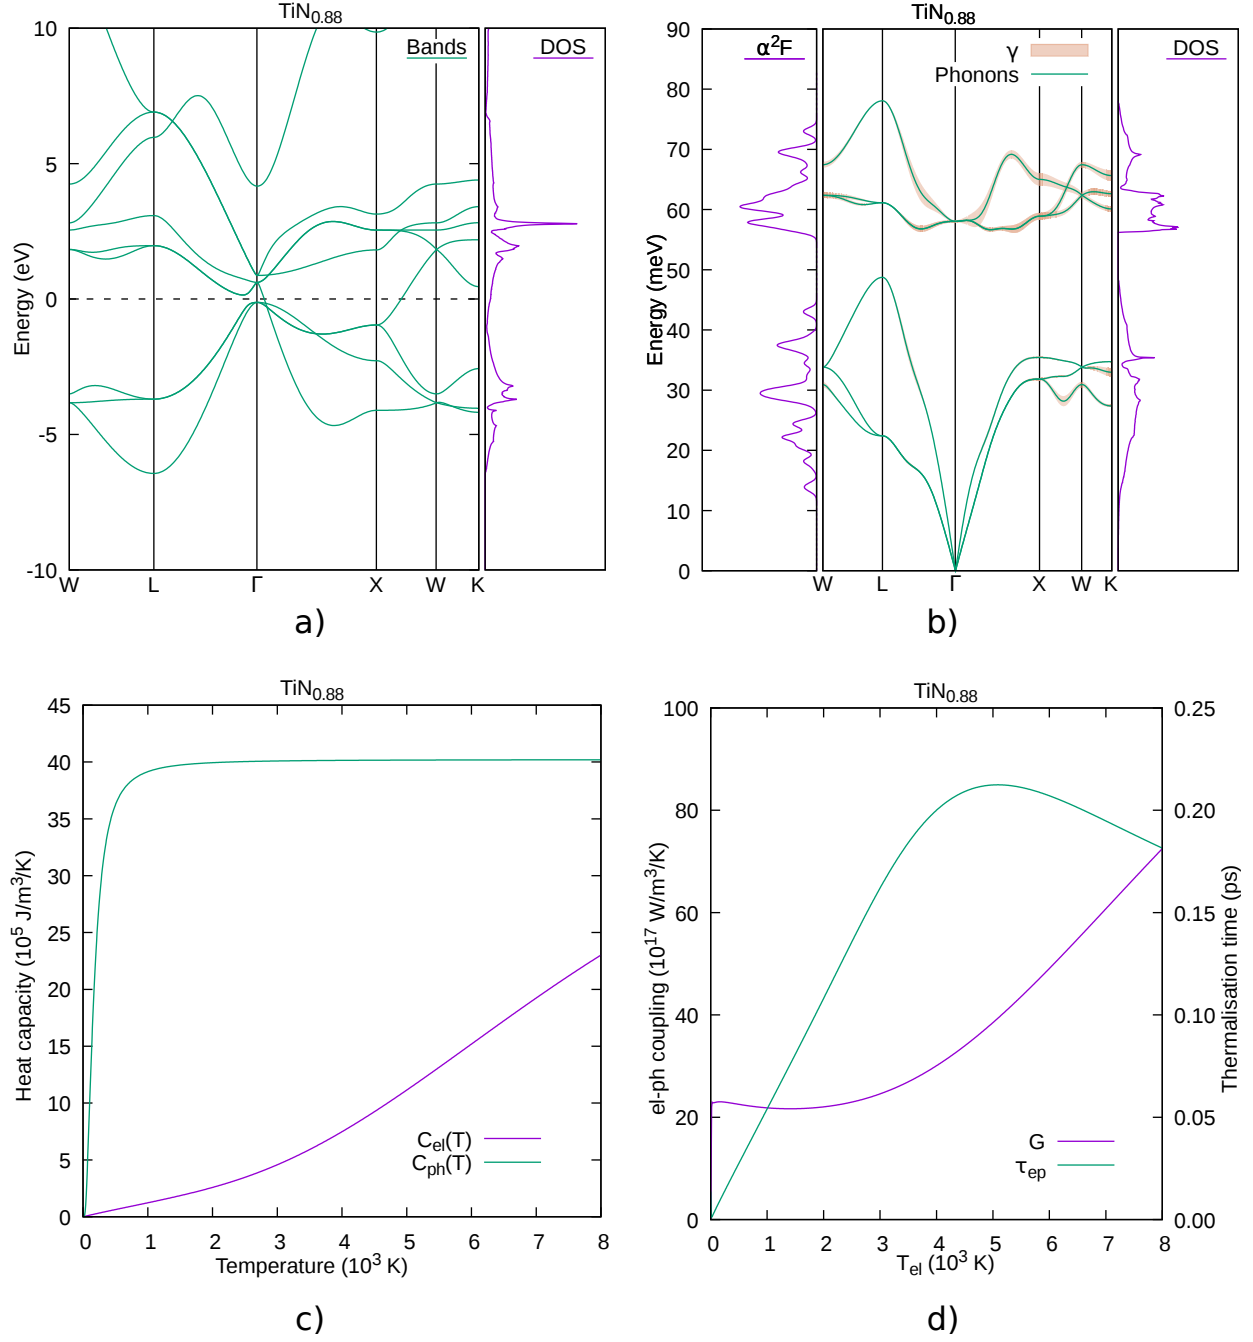

Figure S10: DFT results for  $\text{TiN}_{0.88}$ . a) Electron band structure and DOS (DOS values in the range 0 to 16 states/eV/unitcell). b) Phonon band structure, DOS, phonon linewidths (magnification  $\times 2$ ) and Eliashberg function (DOS and  $\alpha^2F$  in the range 0 to 0.12 states/eV/unitcell and 0 to 1.3, respectively). c) Electron and phonon heat capacities. d) Electron-phonon coupling parameter and hot electron thermalisation time.

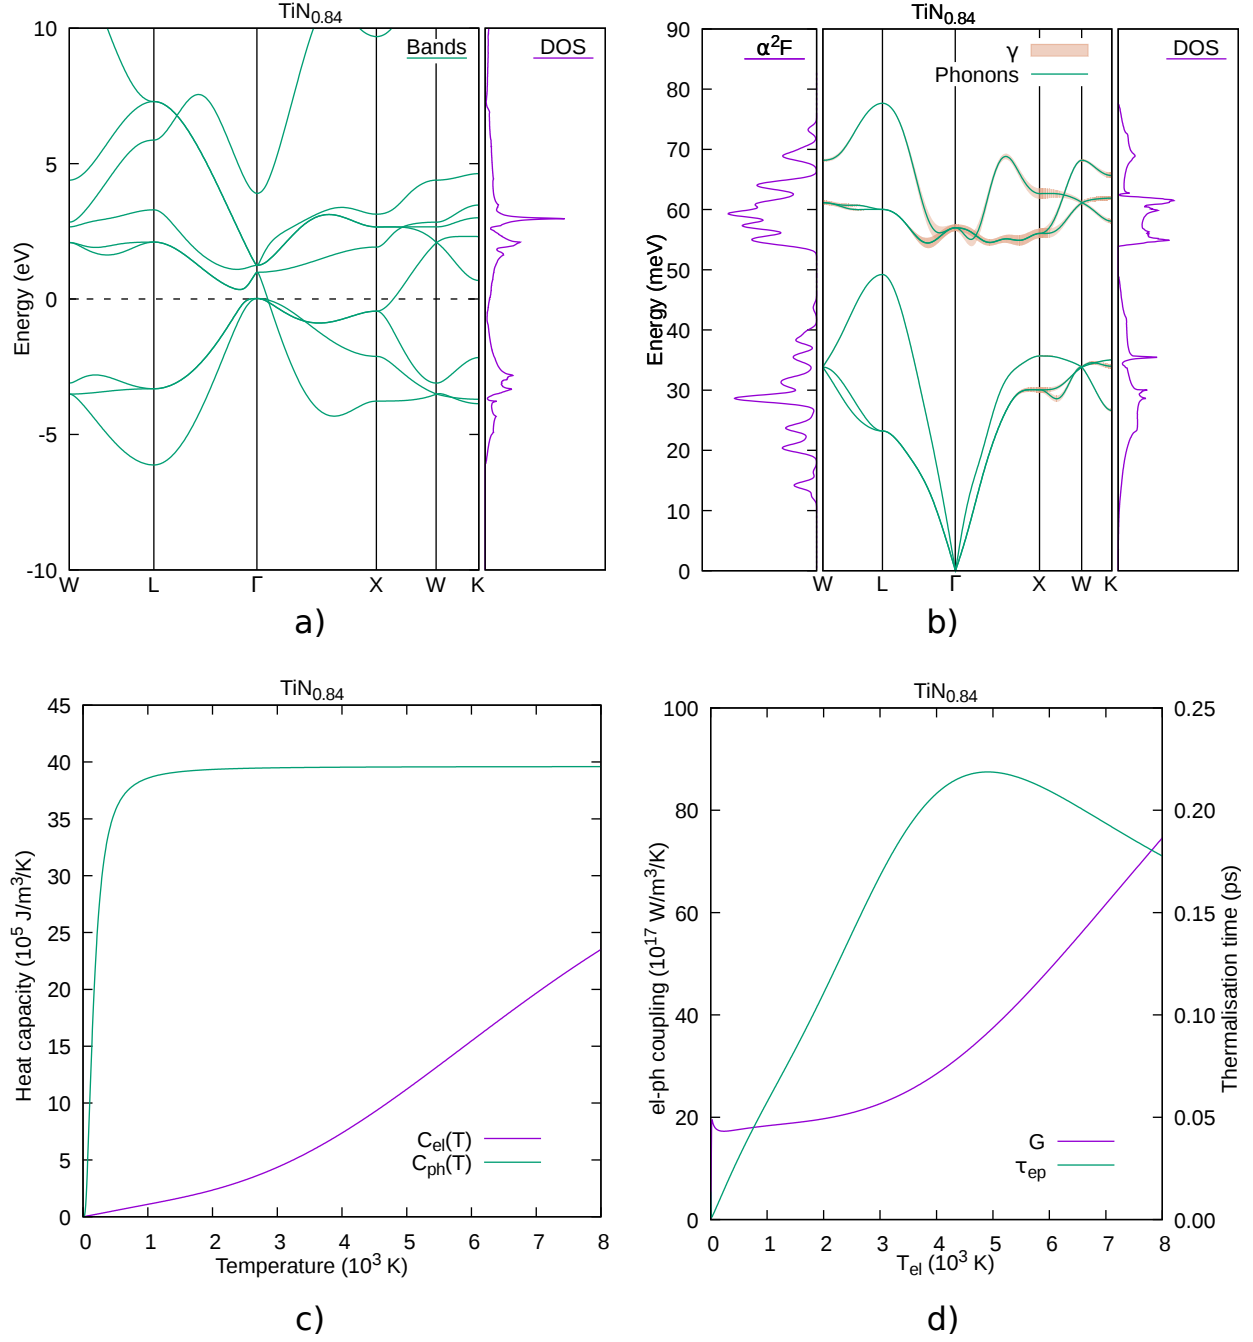

Figure S11: DFT results for  $\text{TiN}_{0.84}$ . a) Electron band structure and DOS (DOS values in the range 0 to 16 states/eV/unitcell). b) Phonon band structure, DOS, phonon linewidths (magnification  $\times 2$ ) and Eliashberg function (DOS and  $\alpha^2F$  in the range 0 to 0.12 states/eV/unitcell and 0 to 1.3, respectively). c) Electron and phonon heat capacities. d) Electron-phonon coupling parameter and hot electron thermalisation time.
